# Supplementary material for: Dynamic Updating of Clinical Survival Prediction Models in a Rapidly Changing Environment
Source: arXiv:2305.00260 ancillary file (2023-04-29)
Supplement: Supplementary file 1 [file SuppInfo_v5_noStyle.pdf]

# Supporting Information for Dynamic Updating of Clinical Survival Prediction Models in a Rapidly Changing Environment

by
**Kamaryn Tanner[1], Ruth H Keogh[1], Carol AC Coupland[2,3], Julia Hippisley-Cox[2], Karla Diaz-Ordaz[4]**

[1]Dept of Medical Statistics, London School of Hygiene and Tropical Medicine, London WC1E 7HT, UK
[2]Nuffield Department of Primary Health Care Sciences, University of Oxford, Oxford OX2 6HT, UK
[3]Centre for Academic Primary Care, School of Medicine, University of Nottingham, Nottingham NG7 2UH, UK
[4]Dept of Statistical Science, University College London, London WC1E 6BT, UK

# Web Appendix A: Simulation study data generation

To simulate data used to evaluate and update the prediction model, i.e. data arriving after development of the original model, we used two different data generating mechanisms: *new cohorts* and *open cohort*. These methods are depicted graphically in Figure 1. Details are provided below.

## New cohorts data

New cohorts data was generated assuming that it would take one year to accumulate data on the same number of individuals as in the original development dataset ($n_{dev} = 10,000$).

For months $w = 1, \ldots, 15$, where $w = 1$ represents the first month after collection of the original development dataset, data was created as follows:

1. Generate a covariate matrix for $n$=10,000/12 unique individuals with $X_1 \sim U(1.8, 9.5)$, $X_2 \sim N(1, 1)$, $X_3 \sim Bern(p_{X_3})$ and $X_4 \sim Bern(p_{X_4,w})$ where $p_{X_4,w}$ may vary by month.

2. For the "New treatment + comorbidity" scenario, we additionally generate an interaction between the new treatment and the comorbidity. Compute $X_5 = X_3 \times X_4$

3. Given log hazard ratios $\beta_1, \beta_2, \beta_3, \beta_4, \beta_5$, and assuming exponentially distributed survival times with baseline rate parameter $\lambda_w$, the hazard of an event at time $t$ can be written $h(t) = \lambda_w \exp(\beta_1 X_1 + \beta_2 X_2 + \beta_3 X_3 + \beta_4 X_4 + \beta_5 X_5)$. Survival times $T$ are generated using the cumulative hazard inversion technique [Bender et al., 2005] and then administrative censoring is applied for each person at $t$=0.25 (3 months). If $T$ <0.25, set the event indicator $E$ to 1, otherwise 0.

These monthly datasets were combined to form quarterly datasets, each with $n$ =2,500 records. See Figure 1-top.

## Open cohort data

Generation of open cohort data required a different procedure. First, a month 1 covariate matrix was generated for 11,000 individuals. As our aim was to have 10,000 people at the start of each period, data was generated for 10,000 people in the open cohort at the beginning plus an additional 1,000 extras used to replace those individuals who had events. The covariate matrix is comprised of: $X_1 \sim U(1.8, 9.5)$, $X_2 \sim N(1, 1)$, $X_3 \sim Bern(p_{X_3})$ and $X_4 \sim Bern(p_{X_{4,1}})$. $X_1$, $X_2$, $X_3$ remain fixed for all months. For the "New treatment + comorbidity" scenario, we also generate the interaction between the comorbidity and the treatment, $X_{5,1} = X_3 \times X_{4,1}$. For months $w = 2, \ldots, 15$:

1. Set $X_{4,w} = 1$ for all individuals with $X_{4,(w-1)} = 1$ to indicate that once an individual is treated, they remain treated in all future months.

2. Based on $p_{X_4,w}$ and other constraints (see Supplementary Information Table S1), set $X_{4,w} = 1$ for a random selection of eligible individuals who were previously untreated, ie. $X_{4,w-1} = 0$. This is used to simulate the introduction of a new treatment that is rolled out to an increasing number of people over time.

3. For the "New treatment + comorbidity" scenario, compute $X_{5,w} = X_3 \times X_{4,w}$

4. Given log hazard ratios $\beta_1, \beta_2, \beta_3, \beta_4, \beta_5$, and assuming exponentially distributed survival times with baseline rate parameter $\lambda_w$, the hazard of an event at time $t$ can be writen $h(t) =$

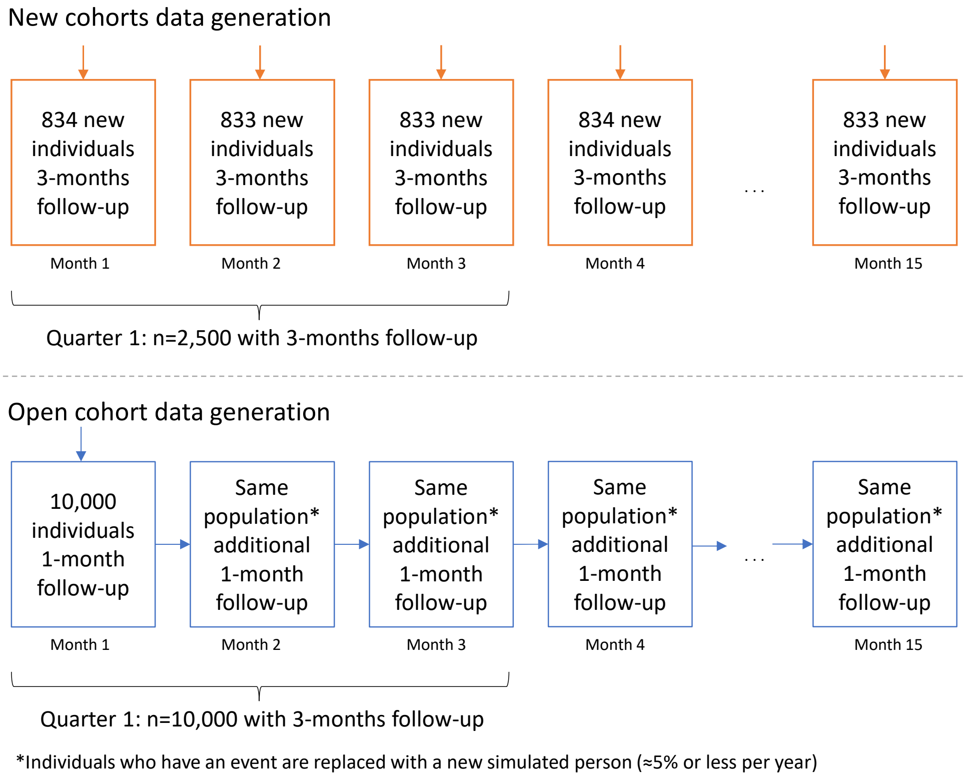


Web Figure 1: Illustration of the two simulated data generation processes. To generate *new cohorts* simulation data (top), new individuals are simulated each month with 3-months of follow-up. This method mimics the situation where individuals have had a certain test result, diagnosis or experience that makes them eligible to be in the modelled population. Generation of *open cohort* data (bottom) begins by simulating an initial population of 10,000 individuals who have additional follow-up time added each month. When individuals experience an event, a new simulated individual is added to replace them. This is similar to data that would be retrieved from electronic health records where the population is essentially fixed but there is some small amount of churn.

$\lambda_w \exp(\beta_1 X_1 + \beta_2 X_2 + \beta_3 X_3 + \beta_4 X_4 + \beta_5 X_5)$. Survival times $T$ are generated using the cumulative hazard inversion technique [Bender et al., 2005] and then administrative censoring is applied for each person at $t$=0.25 (3 months). If $T$ <0.25, set the event indicator $E$ to 1, otherwise 0.

## Number of simulated datasets

Our aim was to detect a difference of 0.01 in the mean c-index with a 5% significance level and 90% power. Using a standard formula based on the normal distribution and assuming a C-index standard deviation of less than 0.05, we need at least 525 simulated datasets. To be conservative, we used $n_{sim}$=600 repetitions.

Web Table 1: Listing of simulation parameters for each scenario. $\lambda$ is the baseline rate parameter, $\beta$s are log hazard ratios and $p_{X_a}$ represents the probability that $X_a$=1.

| Scenario | Baseline parameter ($\lambda$) | log HR ($\beta$) | Value of $p$ |
|---|---|---|---|
| All scenarios | | $\beta_1$ =0.50 | - |
| | | $\beta_2$ =0.75 | - |
| Scenarios with calibration drift | | | |
| Decreasing events | decreasing, range= | $\beta_3$ =-0.25 | $p_{X_3}$ =0.35 |
| | $\lambda_{\text{month1}}$ =0.0007 | $\beta_4$ =NA | $p_{X_4}$ =NA |
| | $\lambda_{\text{month15}}$ =0.00025 | $\beta_5$ =NA | |
| Increasing events | increasing, range= | $\beta_3$ =-0.25 | $p_{X_3}$ =0.35 |
| | $\lambda_{\text{month1}}$ =0.00072 | $\beta_4$ =NA | $p_{X_4}$ =NA |
| | $\lambda_{\text{month15}}$ =0.00137 | $\beta_5$ =NA | |
| Scenario with rare predictor | | | |
| Rare predictor | $\lambda_w$ =0.00065 | $\beta_3$ =0.8 | $p_{X_3}$ increases with $X_1$ |
| | $w = 1, \ldots, 15$ | | $p_{X_3}$ =0.005 if 5.5$\leq X_1$ <6.0 |
| | | | $p_{X_3}$ =0.005 if 6.0$\leq X_1$ <6.5 |
| | | | $p_{X_3}$ =0.01 if 6.5$\leq X_1$ <7.0 |
| | | | $p_{X_3}$ =0.02 if 7.0$\leq X_1$ <7.5 |
| | | | $p_{X_3}$ =0.02 if 7.5$\leq X_1$ <8.0 |
| | | | $p_{X_3}$ =0.03 if 8.0$\leq X_1$ <8.5 |
| | | | $p_{X_3}$ =0.04 if 8.5$\leq X_1$ <9.0 |
| | | | $p_{X_3}$ =0.05 if 9.0$\leq X_1$ |
| | | $\beta_4$ =NA | $p_{X_4}$ =NA |
| Scenarios with new predictors | | | |
| New treatment | $\lambda_w$ =0.001 | $\beta_3$ =NA | $p_{X_3}$ =NA |
| | $w = 1, \ldots, 15$ | $\beta_4$ =-2.3 | $p_{X_4}$ increases with time, $X_1$ |
| | | | $p_{X_{4,4}}$ =0.05 (8.0$\leq X_1$) |
| | | | $p_{X_{4,5}}$ =0.10 (8.0$\leq X_1$) |
| | | | $p_{X_{4,6}}$ =0.15 (7.5$\leq X_1$) |
| | | | $p_{X_{4,7}}$ =0.18 (7.0$\leq X_1$) |
| | | | $p_{X_{4,8}}$ =0.24 (7.0$\leq X_1$) |
| | | | $p_{X_{4,9}}$ =0.30 (6.5$\leq X_1$) |
| | | | $p_{X_{4,10}}$ =0.33 (6.0$\leq X_1$) |
| | | | $p_{X_{4,11}}$ =0.37 (6.0$\leq X_1$) |
| | | | $p_{X_{4,12}}$ =0.45 (5.0$\leq X_1$) |
| | | | $p_{X_{4,13}}$ =0.50 (5.0$\leq X_1$) |
| | | | $p_{X_{4,14}}$ =0.60 (3.0$\leq X_1$) |
| | | | $p_{X_{4,15}}$ =0.675 (3.0$\leq X_1$) |
| New treatment + | decreasing, range= | $\beta_3$ =1.78 | $p_{X_3}$ =0.05 |
| comorbidity | $\lambda_1$ =0.00060 | $\beta_4$ =-1.77 | $p_{X_{4,4}}$ =0.02 (8.0$\leq X_1$ or $X_3 = 1$) |
| | $\lambda_{15}$ =0.00046 | $\beta_5$ =0.26 | $p_{X_{4,5}}$ =0.04 (8.0$\leq X_1$ or $X_3 = 1$) |
| | | | $p_{X_{4,6}}$ =0.07 (8.0$\leq X_1$ or $X_3 = 1$) |
| | | | $p_{X_{4,7}}$ =0.11 (7.0$\leq X_1$ or $X_3 = 1$) |
| | | | $p_{X_{4,8}}$ =0.16 (7.0$\leq X_1$ or $X_3 = 1$) |
| | | | $p_{X_{4,9}}$ =0.25 (7.0$\leq X_1$ or $X_3 = 1$) |
| | | | $p_{X_{4,10}}$ =0.325 (6.0$\leq X_1$ or $X_3 = 1$) |
| | | | $p_{X_{4,11}}$ =0.40 (6.0$\leq X_1$ or $X_3 = 1$) |
| | | | $p_{X_{4,12}}$ =0.475 (5.0$\leq X_1$ or $X_3 = 1$) |
| | | | $p_{X_{4,13}}$ =0.525 (5.0$\leq X_1$ or $X_3 = 1$) |
| | | | $p_{X_{4,14}}$ =0.55 (3.0$\leq X_1$ or $X_3 = 1$) |
| | | | $p_{X_{4,15}}$ =0.575 (3.0$\leq X_1$ or $X_3 = 1$) |

## Web Appendix B: Simulation study results

Web Table 2: Simulation results for the calibration drift scenario with decreasing event rate for both open cohort (left) and new cohorts (right) simulated datasets. For each updating method and dataset type, the C-index, calibration intercept, calibration slope, and Brier score over 600 simulated datasets is shown for a model updated quarterly over one year. Monte Carlo standard error was <0.005 for all data points. Bold text indicates that a method was significantly better than all other methods ($p < 0.05$) for that evaluation metric using a Wilcoxon signed rank test.

| **Open Cohort/Decreasing event rate** | | | | | **New Cohorts/Decreasing event rate** | | | | |
|---|---|---|---|---|---|---|---|---|---|
| | Predictions on data from: | | | | | Predictions on data from: | | | |
| C-index | Q2 | Q3 | Q4 | Q5 | C-index | Q2 | Q3 | Q4 | Q5 |
| No update | 0.81 | 0.81 | 0.81 | 0.81 | No update | 0.82 | 0.81 | 0.81 | 0.81 |
| Recal always | 0.81 | 0.81 | 0.81 | 0.81 | Recal always | 0.82 | 0.81 | 0.81 | 0.81 |
| Refit always | **0.81** | **0.81** | 0.81 | **0.81** | Refit always | 0.81 | 0.81 | 0.81 | 0.80 |
| Bayesian | 0.81 | 0.81 | 0.81 | 0.81 | Bayesian | 0.82 | 0.82 | 0.81 | 0.81 |
| Calibration intercept | Q2 | Q3 | Q4 | Q5 | Calibration intercept | Q2 | Q3 | Q4 | Q5 |
| No update | -0.03 | -0.22 | -0.49 | -0.88 | No update | -0.03 | -0.22 | -0.51 | -0.90 |
| Recal always | 0.06 | **-0.08** | **-0.16** | **-0.26** | Recal always | 0.04 | **-0.12** | **-0.22** | **-0.35** |
| Refit always | -0.03 | -0.18 | -0.28 | -0.39 | Refit always | -0.03 | -0.19 | -0.29 | -0.40 |
| Bayesian | -0.02 | -0.18 | -0.27 | -0.38 | Bayesian | -0.01 | -0.17 | -0.27 | -0.37 |
| Calibration slope | Q2 | Q3 | Q4 | Q5 | Calibration slope | Q2 | Q3 | Q4 | Q5 |
| No update | 1.00 | 0.99 | 1.01 | 1.00 | No update | 1.01 | 1.01 | 1.01 | 1.01 |
| Recal always | 1.00 | 0.99 | 1.01 | 1.00 | Recal always | 1.01 | 1.01 | 1.01 | 1.01 |
| Refit always | 1.00 | 0.98 | 1.01 | 0.99 | Refit always | 0.98 | 0.97 | 0.96 | 0.96 |
| Bayesian | 1.00 | 0.99 | 1.01 | 1.00 | Bayesian | 1.01 | 1.01 | 1.00 | 1.01 |
| Brier score | Q2 | Q3 | Q4 | Q5 | Brier score | Q2 | Q3 | Q4 | Q5 |
| No update | 0.01 | 0.01 | 0.01 | 0.00 | No update | 0.01 | 0.01 | 0.01 | 0.01 |
| Recal always | 0.01 | 0.01 | 0.01 | 0.00 | Recal always | 0.01 | 0.01 | 0.01 | 0.01 |
| Refit always | 0.01 | 0.01 | 0.01 | 0.00 | Refit always | 0.01 | 0.01 | 0.01 | 0.01 |
| Bayesian | 0.01 | 0.01 | 0.01 | 0.00 | Bayesian | 0.01 | 0.01 | 0.01 | 0.01 |

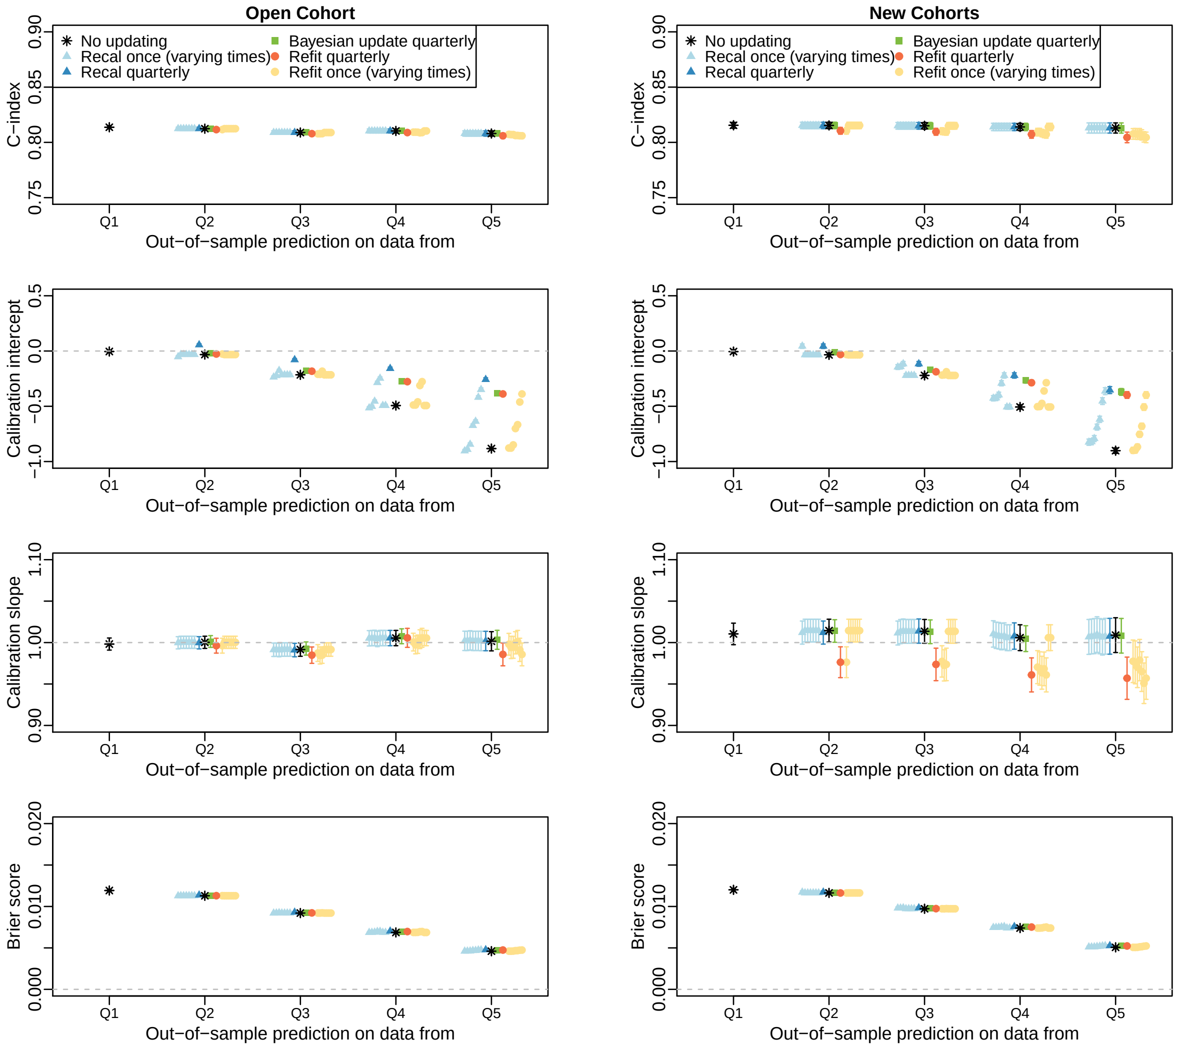


Web Figure 2: Simulation results for the calibration drift scenario with decreasing event rate for both open cohort (left) and new cohorts (right) simulated datasets. Best possible values for calibration intercept, calibration slope and Brier score are indicated with gray dashed lines. Results for ‘Recal once’ and ‘Refit once’ strategies are ordered by update time with the earliest time on the left.

Web Table 3: Simulation results for the calibration drift scenario with increasing event rate for both open cohort (left) and new cohorts (right) simulated datasets. For each updating method and dataset type, the C-index, calibration intercept, calibration slope, and Brier score over 600 simulated datasets is shown for a model updated quarterly over one year. Monte Carlo standard error was <0.005 for all data points. Bold text indicates that a method was significantly better than all other methods ($p < 0.05$) for that evaluation metric using a Wilcoxon signed rank test.

| **Open Cohort/Increasing event rate** | | | | | **New Cohorts/Increasing event rate** | | | | |
|---|---|---|---|---|---|---|---|---|---|
| | Predictions on data from: | | | | | Predictions on data from: | | | |
| C-index | Q2 | Q3 | Q4 | Q5 | C-index | Q2 | Q3 | Q4 | Q5 |
| No update | 0.81 | 0.81 | 0.81 | 0.81 | No update | 0.82 | 0.81 | 0.81 | 0.81 |
| Recal always | 0.81 | 0.81 | 0.81 | 0.81 | Recal always | 0.82 | 0.81 | 0.81 | 0.81 |
| Refit always | 0.81 | 0.81 | 0.81 | 0.81 | Refit always | 0.81 | 0.81 | 0.81 | 0.81 |
| Bayesian | **0.81** | **0.81** | **0.81** | **0.81** | Bayesian | 0.82 | 0.81 | **0.81** | 0.81 |
| Calibration intercept | Q2 | Q3 | Q4 | Q5 | Calibration intercept | Q2 | Q3 | Q4 | Q5 |
| No update | 0.09 | 0.36 | 0.49 | 0.60 | No update | 0.05 | 0.23 | 0.34 | 0.40 |
| Recal always | 0.18 | 0.37 | 0.26 | 0.27 | Recal always | 0.13 | 0.26 | 0.19 | 0.15 |
| Refit always | 0.10 | **0.27** | **0.13** | **0.11** | Refit always | 0.05 | **0.18** | **0.11** | **0.06** |
| Bayesian | 0.10 | 0.27 | 0.13 | 0.11 | Bayesian | 0.07 | 0.20 | 0.12 | 0.08 |
| Calibration slope | Q2 | Q3 | Q4 | Q5 | Calibration slope | Q2 | Q3 | Q4 | Q5 |
| No update | 1.00 | 1.00 | 1.00 | 1.00 | No update | 1.01 | 1.01 | 1.00 | 1.01 |
| Recal always | 1.00 | 1.00 | 1.01 | 1.00 | Recal always | 1.01 | 1.01 | 1.00 | 1.00 |
| Refit always | 0.99 | 0.99 | 1.00 | 0.99 | Refit always | 0.98 | 0.97 | 0.97 | 0.99 |
| Bayesian | 1.00 | 1.00 | 1.01 | 1.00 | Bayesian | 1.01 | 1.01 | 1.00 | 1.01 |
| Brier score | Q2 | Q3 | Q4 | Q5 | Brier score | Q2 | Q3 | Q4 | Q5 |
| No update | 0.01 | 0.02 | 0.02 | 0.02 | No update | 0.01 | 0.02 | 0.02 | 0.02 |
| Recal always | 0.01 | 0.02 | 0.02 | 0.02 | Recal always | 0.01 | 0.02 | 0.02 | 0.02 |
| Refit always | 0.01 | **0.02** | **0.02** | **0.02** | Refit always | 0.01 | **0.02** | 0.02 | 0.02 |
| Bayesian | 0.01 | 0.02 | 0.02 | 0.02 | Bayesian | 0.01 | 0.02 | 0.02 | 0.02 |

Web Table 4: Simulation results for rare predictor scenario with 1% having a risk factor for an event for both open cohort (left) and new cohorts (right) simulated datasets. For each updating method and dataset type, the C-index, calibration intercept and slope, and Brier score over 600 simulated datasets is shown for a model updated quarterly over one year. Monte Carlo standard error was <0.005 for all data points. Bold text indicates that a method was significantly better than all other methods ($p < 0.05$) for that evaluation metric using a Wilcoxon signed rank test.

| **Open Cohort/Rare-1%** | | | | | | **New Cohorts/Rare-1%** | | | | |
|---|---|---|---|---|---|---|---|---|---|---|
| | Predictions on data from: | | | | | | Predictions on data from: | | | |
| C-index | Q2 | Q3 | Q4 | Q5 | | C-index | Q2 | Q3 | Q4 | Q5 |
| No update | 0.82 | 0.81 | 0.81 | 0.81 | | No update | 0.82 | 0.82 | 0.82 | 0.82 |
| Recal always | 0.82 | 0.81 | 0.81 | 0.81 | | Recal always | 0.82 | 0.82 | 0.82 | 0.82 |
| Refit always | 0.81 | 0.81 | 0.81 | 0.81 | | Refit always | 0.82 | 0.81 | 0.82 | 0.82 |
| Bayesian | **0.82** | **0.81** | **0.81** | **0.81** | | Bayesian | 0.82 | 0.82 | 0.82 | 0.82 |
| Calibration intercept | Q2 | Q3 | Q4 | Q5 | | Calibration intercept | Q2 | Q3 | Q4 | Q5 |
| No update | 0.00 | -0.00 | -0.01 | -0.00 | | No update | -0.01 | -0.02 | -0.01 | -0.02 |
| Recal always | 0.00 | 0.00 | 0.02 | 0.06 | | Recal always | -0.01 | -0.03 | -0.01 | -0.03 |
| Refit always | 0.01 | -0.01 | -0.00 | 0.01 | | Refit always | -0.01 | -0.03 | -0.02 | -0.02 |
| Bayesian | 0.02 | -0.00 | -0.00 | 0.01 | | Bayesian | 0.02 | 0.01 | 0.02 | 0.01 |
| Calibration slope | Q2 | Q3 | Q4 | Q5 | | Calibration slope | Q2 | Q3 | Q4 | Q5 |
| No update | 1.00 | 1.00 | 1.00 | 1.00 | | No update | 1.01 | 1.00 | 1.02 | 1.03 |
| Recal always | 1.00 | 1.00 | 1.00 | 1.00 | | Recal always | 1.01 | 1.00 | 1.01 | 1.02 |
| Refit always | 1.00 | 1.00 | 0.99 | 0.99 | | Refit always | 0.98 | 0.97 | 0.98 | 0.99 |
| Bayesian | 1.00 | 1.01 | 1.00 | 1.00 | | Bayesian | 1.01 | 1.00 | 1.02 | 1.02 |
| Brier score | Q2 | Q3 | Q4 | Q5 | | Brier score | Q2 | Q3 | Q4 | Q5 |
| No update | 0.01 | 0.01 | 0.01 | 0.01 | | No update | 0.01 | 0.01 | 0.01 | 0.01 |
| Recal always | 0.01 | 0.01 | 0.01 | 0.01 | | Recal always | 0.01 | 0.01 | 0.01 | 0.01 |
| Refit always | 0.01 | 0.01 | 0.01 | 0.01 | | Refit always | 0.01 | **0.01** | **0.01** | **0.01** |
| Bayesian | 0.01 | 0.01 | 0.01 | 0.01 | | Bayesian | 0.01 | 0.01 | 0.01 | 0.01 |

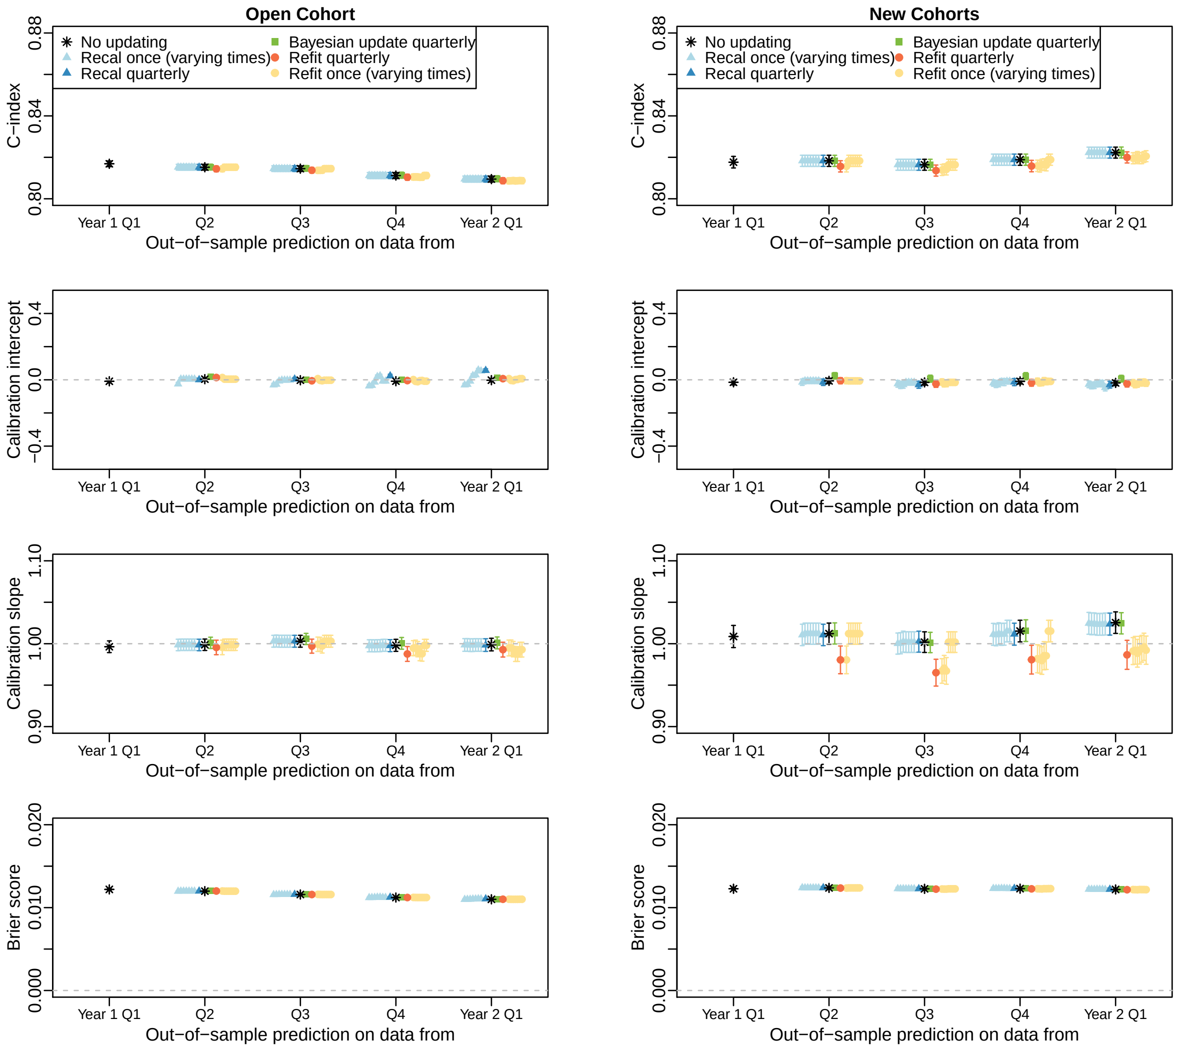


Web Figure 3: Simulation results for the rare predictor scenario where 1% of the population is at increased risk for an event. Open cohort (left) and new cohorts (right) simulated datasets are shown. Best possible values for calibration intercept, calibration slope and Brier score are indicated with gray dashed lines. Results for 'Recal once' and 'Refit once' strategies are ordered by update time with the earliest time on the left.

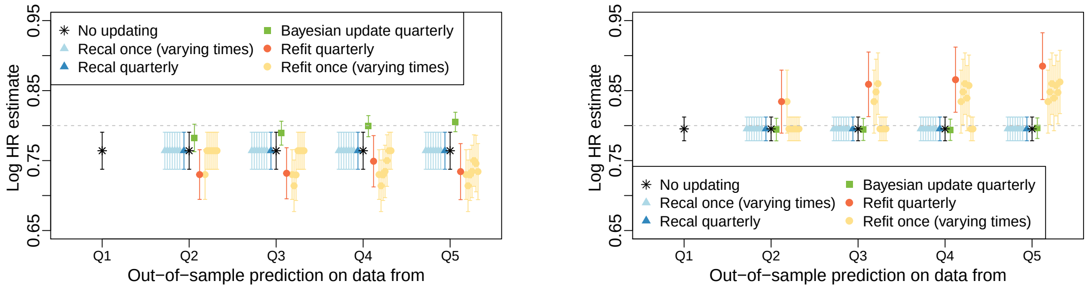


Web Figure 4: Average estimated log hazard ratio (HR) for the rare risk factor for the scenario where 1% of the population has a risk factor for an event. On the left, results for the open cohort simulation; on the right, results for the new cohorts simulation. The true log hazard ratio is shown by the gray dashed line. Results for 'Recal once' and 'Refit once' strategies are ordered by update time with the earliest time on the left.

Web Table 5: Simulation results for the new treatment scenario for both open cohort (left) and new cohorts (right) simulated datasets. For each updating method and dataset type, the C-index, calibration intercept, calibration slope, and Brier score over 600 simulated datasets is shown for a model updated quarterly over one year. Monte Carlo standard error was <0.005 for all data points. Bold text indicates that a method was significantly better than all other methods ($p < 0.05$) for that evaluation metric using a Wilcoxon signed rank test.

| **Open Cohort/New treatment** | | | | | **New Cohorts/New treatment** | | | | |
|---|---|---|---|---|---|---|---|---|---|
| | Predictions on data from: | | | | | Predictions on data from: | | | |
| C-index | Q2 | Q3 | Q4 | Q5 | C-index | Q2 | Q3 | Q4 | Q5 |
| No update | 0.78 | 0.73 | 0.68 | 0.66 | No update | 0.78 | 0.75 | 0.74 | 0.77 |
| Recal always | 0.78 | 0.73 | 0.68 | 0.66 | Recal always | 0.78 | 0.75 | 0.74 | 0.77 |
| Refit always | 0.78 | 0.75 | 0.73 | 0.73 | Refit always | 0.78 | 0.80 | 0.81 | 0.84 |
| Bayesian | **0.78** | **0.75** | 0.72 | 0.72 | Bayesian | 0.78 | **0.81** | **0.82** | **0.85** |
| Calibration intercept | Q2 | Q3 | Q4 | Q5 | Calibration intercept | Q2 | Q3 | Q4 | Q5 |
| No update | -0.26 | -0.67 | -1.08 | -1.56 | No update | -0.29 | -0.66 | -0.96 | -1.17 |
| Recal always | -0.27 | -0.38 | -0.36 | -0.43 | Recal always | -0.26 | -0.38 | -0.33 | -0.26 |
| Refit always | -0.27 | -0.17 | **-0.17** | **-0.20** | Refit always | -0.27 | 0.00 | -0.01 | 0.00 |
| Bayesian | -0.27 | **-0.16** | -0.19 | -0.23 | Bayesian | **-0.26** | 0.01 | 0.02 | 0.04 |
| Calibration slope | Q2 | Q3 | Q4 | Q5 | Calibration slope | Q2 | Q3 | Q4 | Q5 |
| No update | 0.85 | 0.66 | 0.50 | 0.48 | No update | 0.88 | 0.73 | 0.73 | 0.85 |
| Recal always | 0.85 | 0.66 | 0.50 | 0.48 | Recal always | 0.88 | 0.73 | 0.73 | 0.85 |
| Refit always | 0.85 | 0.93 | **0.91** | **0.95** | Refit always | 0.87 | 0.80 | 0.93 | 0.96 |
| Bayesian | 0.85 | **0.93** | 0.85 | 0.83 | Bayesian | 0.88 | **0.98** | **0.99** | **1.00** |
| Brier score | Q2 | Q3 | Q4 | Q5 | Brier score | Q2 | Q3 | Q4 | Q5 |
| No update | 0.01 | 0.01 | 0.01 | 0.00 | No update | 0.01 | 0.01 | 0.01 | 0.01 |
| Recal always | 0.01 | 0.01 | 0.01 | 0.00 | Recal always | 0.01 | 0.01 | 0.01 | 0.01 |
| Refit always | 0.01 | 0.01 | 0.01 | 0.00 | Refit always | 0.01 | 0.01 | 0.01 | 0.01 |
| Bayesian | 0.01 | 0.01 | 0.01 | 0.00 | Bayesian | 0.01 | 0.01 | 0.01 | 0.01 |

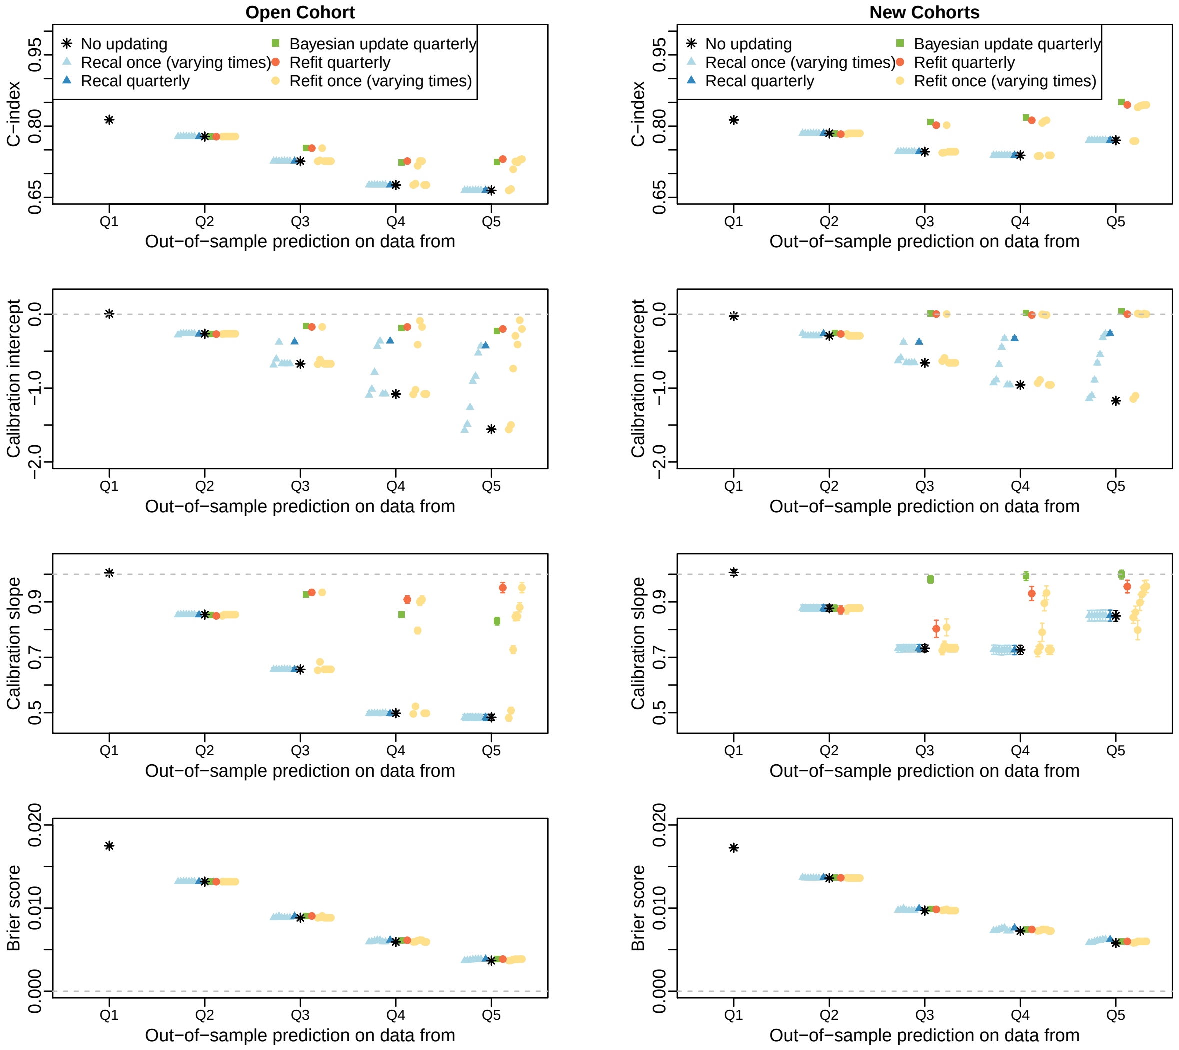


Web Figure 5: Simulation results for the scenario where a new treatment was introduced in Q2. On the left, results for the open cohort simulation; on the right, results for the new cohorts simulation. Best possible values for calibration intercept, calibration slope and Brier score are indicated with gray dashed lines. Results for 'Recal once' and 'Refit once' strategies are ordered by update time with the earliest time on the left.

Web Table 6: Simulation results for the new treatment + comorbidity scenario for both open cohort (left) and new cohorts (right) simulated datasets. For each updating method and dataset type, the C-index, calibration intercept, calibration slope, and Brier score over 600 simulated datasets is shown for a model updated quarterly over one year. Monte Carlo standard error was <0.005 for all data points. Bold text indicates that a method was significantly better than all other methods ($p < 0.05$) for that evaluation metric using a Wilcoxon signed rank test.

| **Open Cohort/New treatment + comorbidity** | | | | | **New Cohorts/New treatment + comorbidity** | | | | |
|---|---|---|---|---|---|---|---|---|---|
| | Predictions on data from: | | | | | Predictions on data from: | | | |
| C-index | Q2 | Q3 | Q4 | Q5 | C-index | Q2 | Q3 | Q4 | Q5 |
| No update | 0.82 | 0.79 | 0.74 | 0.72 | No update | 0.82 | 0.80 | 0.78 | 0.81 |
| Recal always | 0.82 | 0.79 | 0.74 | 0.72 | Recal always | 0.82 | 0.80 | 0.78 | 0.81 |
| Refit always | 0.82 | 0.79 | 0.76 | 0.76 | Refit always | 0.82 | 0.80 | 0.79 | 0.83 |
| Bayesian | **0.82** | **0.79** | **0.76** | **0.76** | Bayesian | 0.82 | **0.82** | **0.81** | **0.84** |
| Calibration intercept | Q2 | Q3 | Q4 | Q5 | Calibration intercept | Q2 | Q3 | Q4 | Q5 |
| No update | -0.16 | -0.51 | -1.11 | -1.50 | No update | -0.18 | -0.52 | -1.04 | -1.18 |
| Recal always | -0.25 | -0.41 | -0.65 | -0.44 | Recal always | -0.23 | -0.43 | -0.63 | -0.30 |
| Refit always | -0.15 | -0.12 | -0.35 | -0.42 | Refit always | -0.15 | -0.48 | -0.71 | -0.58 |
| Bayesian | **-0.14** | **-0.09** | **-0.33** | **-0.28** | Bayesian | -0.13 | **-0.03** | **0.01** | **-0.04** |
| Calibration slope | Q2 | Q3 | Q4 | Q5 | Calibration slope | Q2 | Q3 | Q4 | Q5 |
| No update | 0.96 | 0.85 | 0.69 | 0.68 | No update | 0.97 | 0.90 | 0.82 | 0.92 |
| Recal always | 0.96 | 0.85 | 0.69 | 0.68 | Recal always | 0.97 | 0.90 | 0.82 | 0.92 |
| Refit always | 0.96 | 0.94 | 0.89 | 0.93 | Refit always | 0.95 | 0.89 | 0.85 | 0.91 |
| Bayesian | 0.96 | **0.95** | **0.89** | **0.93** | Bayesian | 0.97 | **0.98** | **0.94** | **0.96** |
| Brier score | Q2 | Q3 | Q4 | Q5 | Brier score | Q2 | Q3 | Q4 | Q5 |
| No update | 0.01 | 0.01 | 0.00 | 0.00 | No update | 0.01 | 0.01 | 0.00 | 0.00 |
| Recal always | 0.01 | 0.01 | 0.00 | 0.00 | Recal always | 0.01 | 0.01 | 0.01 | 0.00 |
| Refit always | 0.01 | 0.01 | 0.00 | 0.00 | Refit always | 0.01 | 0.01 | 0.00 | 0.00 |
| Bayesian | 0.01 | 0.01 | 0.00 | 0.00 | Bayesian | 0.01 | 0.01 | 0.01 | 0.00 |

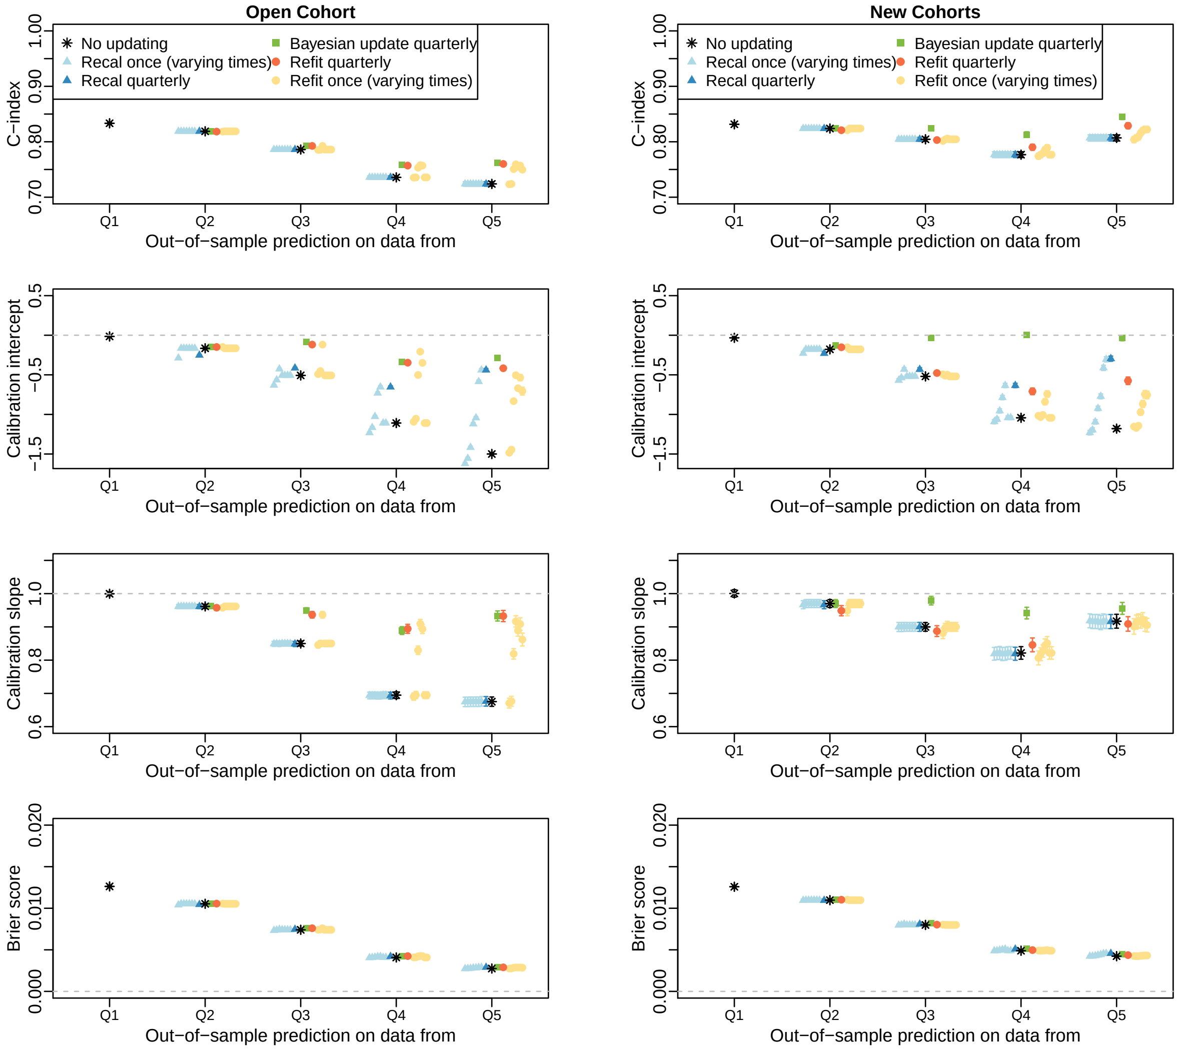


Web Figure 6: Simulation results for the new treatment + comorbidity scenario. On the left, results for the open cohort simulation; on the right, results for the new cohorts simulation. Best possible values for calibration intercept, calibration slope and Brier score are indicated with gray dashed lines. Results for 'Recal once' and 'Refit once' strategies are ordered by update time with the earliest time on the left.

# Web Appendix C: Sensitivity analysis on forgetting factor

We used a fixed population simulation with the new treatment scenario to investigate the impact of different values of $\xi$, the forgetting factor in Bayesian dynamic updating, in a scenario with an abrupt change. Figure 7 shows the log hazard ratio estimates for the continuous covariate $x1$ (left) and for treatment (right) after its introduction in the second quarter. For both, at all time points, the Bayesian estimated log hazard ratios when the forgetting factor is 0.01 are virtually the same as those estimated using the refit strategy. Conversely, when the forgetting factor is high (0.99 or 0.9), the estimates move more slowly away from the original model or prior. At the third and fourth prediction times, the calibration intercept was closer to zero for updates with lower values of $\xi$ but absolute differences between the methods were less than 0.06.

Revisiting the decreasing event rate scenario where only the baseline hazard changed over time, the analysis was insensitive to the choice of $\xi$ for values of 0.5, 0.9, and 0.99 with all three having indistinguishable calibration intercept and slope, C-index and Brier score for all updates.

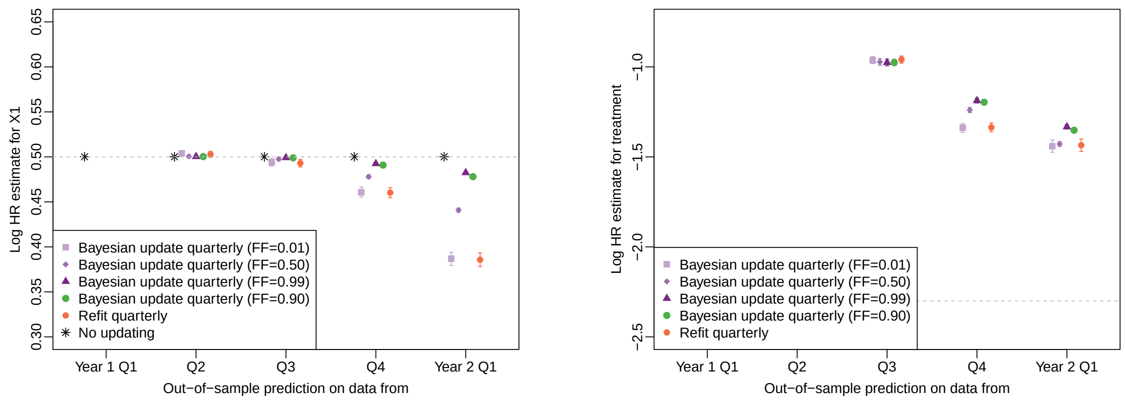


Web Figure 7: Simulation results for the new treatment scenario when the quarterly Bayesian updating used different forgetting factors (FF). On the left, log hazard ratio (HR) estimates for $X_1$, a continuous covariate similar to age are shown. On the right, log HR estimates for treatment. Treatment was introduced at the beginning of Q2 to the elderly first and then to individuals with progressively lower values of $X_1$. Because the original model did not include treatment, there is no log HR estimate for treatment for no updating. A forgetting factor close to zero (close to 1) equates to greater (less) uncertainty in the prior used in the updated Bayesian model.

## Web Appendix D: Study population characteristics

Web Table 7: Characteristics of the total study population ($n$=1,000,000) at the study period start date. Number (percent) are presented or median (IQR) for age and body mass index. To calculate age, all individuals are assumed to have a birthdate of 1 July.

| **Characteristics** | | **Total cohort** | |
|---|---|---|---|
| Age (years) | median (IQR) | 45 | (31-61) |
| Body mass index (kg/m$^2$) | median (IQR) | 25.5 | (22.5-29.2) |
| | missing | 184,213 | (18.4) |
| Sex | Male | 497,679 | (49.8) |
| | Female | 502,321 | (50.2) |
| Type 1 diabetes | No | 994,378 | (99.4) |
| | Yes | 5,622 | (0.6) |
| Chronic obstructive pulmonary disease (COPD) | No | 977,874 | (97.8) |
| | Yes | 22,126 | (2.2) |
| Dementia | No | 989,957 | (99.0) |
| | Yes | 10,043 | (1.0) |
| Region | East Midlands | 24,657 | (2.5) |
| | East of England | 37,220 | (3.7) |
| | London | 256,070 | (25.6) |
| | North East | 22,514 | (2.3) |
| | North West | 180,088 | (18.0) |
| | South Central | 122,748 | (12.3) |
| | South East | 118,690 | (11.9) |
| | South West | 99,519 | (10.0) |
| | West Midlands | 101,810 | (10.2) |
| | Yorkshire & Humber | 36,684 | (3.7) |

## References


R. Bender, T. Augustin, and M. Blettner. Generating survival times to simulate cox proportional hazards models. *Statistics in Medicine*, 24:1713–1723, 2005. doi: 10.1002/sim.2059.
